# Supplementary material for: Uniformly Area Expanding Flows in Spacetimes
Source: arXiv:1508.03779 source file (2015-08-16)
Supplement: Supplementary file 1 [file appendix2.tex]

\chapter{Geometric Objects}
\label{chap:geometric objects}

Let $(M^{n}, g)$ be a Riemannian manifold. We now define some geometric objects

\item The Riemann curvature operator $R$ acts on vector fields $X, Y, Z \in \Gamma(TM)$ as follows:
\begin{equation}\label{Riemann curvature operator}
R(X, Y)Z = D_{X}D_{Y}Z - D_{Y}D_{X}Z - D_{[X, Y]}Z.
\end{equation}
We can thus define a $(1, 3)$ tensor field $R = R^{k}_{lij} dx^{l} \otimes dx^{i} \otimes dx^{j}\otimes \frac{\p}{\p x^{k}}$, such that 
\[R(\frac{\p}{\p x^{i}}, \frac{\p}{\p x^{j}})\frac{\p}{\p x^{l}} =: R^{k}_{lij}\frac{\p}{\p x^{k}}.\]
One can verify that 
\begin{equation}\label{components of Riemann curvature operator}
R^{k}_{lij} = \frac{\p \Gamma^{k}_{jl}}{\p x^{i}} - \frac{\Gamma^{k}_{il}}{\p x^{j}} + \Gamma^{k}_{im}\Gamma^{m}_{jl} - \Gamma^{k}_{jm}\Gamma^{m}_{il}.
\end{equation}

Using the metric $g$, we can define a new $(0, 4)$ tensor field $Rm\footnote{There are different definitions of the Riemann curvature tensor, all up to a sign. We have adopted the convention from the book ''\emph{Riemannian Geometry and Geometric Analysis, 5th edition}'' by Jost.}: = R_{klij}dx^{k}\otimes dx^{l}\otimes dx^{i}\otimes dx^{j}$ with components $R_{klij}: = g_{km}R^{m}_{lij}$. One verifies that
\[R_{klij} = \<R(\p_{i}, \p_{j})\p_{l}, \p_{k}\>.\]
$Rm$ is called the Riemannian curvature tensor with respect to the metric $g$.
We have the second Bianchi identity:
\begin{equation}\label{second Bianchi identity}
R_{klij, h} + R_{lhij,k} + R_{hkij,l}  = 0, \quad \forall k,l,i,j,h.
\end{equation}
 
\item We now define the associated intrinsic curvatures on $(M,g)$. The sectional curvature of the plane spanned by the linearly independent tangent vectors $X = a^{i}\p_{i}|_{p}, Y = b^{j}\p_{j}|_{p} \in T_{p}M$ is 
\begin{align}
K(X\wedge Y)& : = \frac{\<R(X, Y)Y, X\>}{|X\wedge Y|^{2}}\notag \\
&  = \frac{\<R(a^{i}\frac{\p}{\p x^{i}}, b^{j}\frac{\p}{\p x^{j}})b^{k}\frac{\p}{\p x^{k}}, a^{l}\frac{\p}{\p x^{l}}\>}{g_{ik}g_{jl}(a^{i}a^{k}b^{j}b^{l} - a^{i}a^{j}b^{k}b^{l})}\notag \\
& = \frac{R_{lkij}a^{i}b^{j}a^{l}b^{k}}{g_{ik}g_{jl}(a^{i}a^{k}b^{j}b^{l} - a^{i}a^{j}b^{k}b^{l})}\notag \\
& = \frac{R_{ijkl}a^{i}b^{j}a^{k}b^{l}}{(g_{ik}g_{jl} - g_{ij}g_{kl}) a^{i}b^{j}a^{k}b^{l}}, \label{sectional curvature}
\end{align}
where $|X\wedge Y|^{2}: = \<X, X\>\cdot \<Y,Y\> - \<X, Y\>^{2}$.

The Ricci curvature in the direction $X\in T_{p}M$ is given by
\begin{equation}
\text{Ric}(X, X): = g^{jl}\<R(X, \frac{\p}{\p x^{j}})\frac{\p}{\p x^{l}}, X\>.
\end{equation}
Therefore the Ricci curvature tensor is given by the (2,4)-contraction of the Riemann curvature tensor, i.e., 
\begin{align}
\text{Ric}_{ij} & = \text{Ric}(\frac{\p}{\p x^{i}}, \frac{\p}{\p x^{j}}) = g^{kl}\<R(\frac{\p}{\p x^{i}}, \frac{\p}{\p x^{k} })\frac{\p}{\p x^{l}}, \frac{\p}{\p x^{j}}\> = g^{kl}R{jlik} = g^{kl}R_{ikjl} = -R^{l}_{ijl}\notag \\
& = \frac{\p\Gamma^{k}_{ij}} {\p x^{k}} - \frac{\p\Gamma^{k}_{ik}}{\p x^{j}} + \Gamma^{k}_{kl}\Gamma^{l}_{ij} - \Gamma^{k}_{jl}\Gamma^{l}_{ik}. \label{Ricci curvature tensor}
\end{align}

The scalar curvature is
\begin{equation}\label{scalar curvature tensor}
R: = g^{ij}\text{Ric}_{ij}.
\end{equation}
Thus the Ricci curvature in the direction $X$ is the average of the sectional curvature of all planes in $T_{p}M$ containing $X$, and the scalar curvature is the average of the Ricci curvature of all unit vectors, i.e., of the sectional curvature of all planes in $T_{p}M$.
